# Supplementary material for: VolumeDiffusion: Flexible Text-to-3D Generation with Efficient Volumetric Encoder
Source: arXiv:2312.11459 source file (2024-08-13)
Supplement: Supplementary file 1 [file fig_supplementary.pdf]

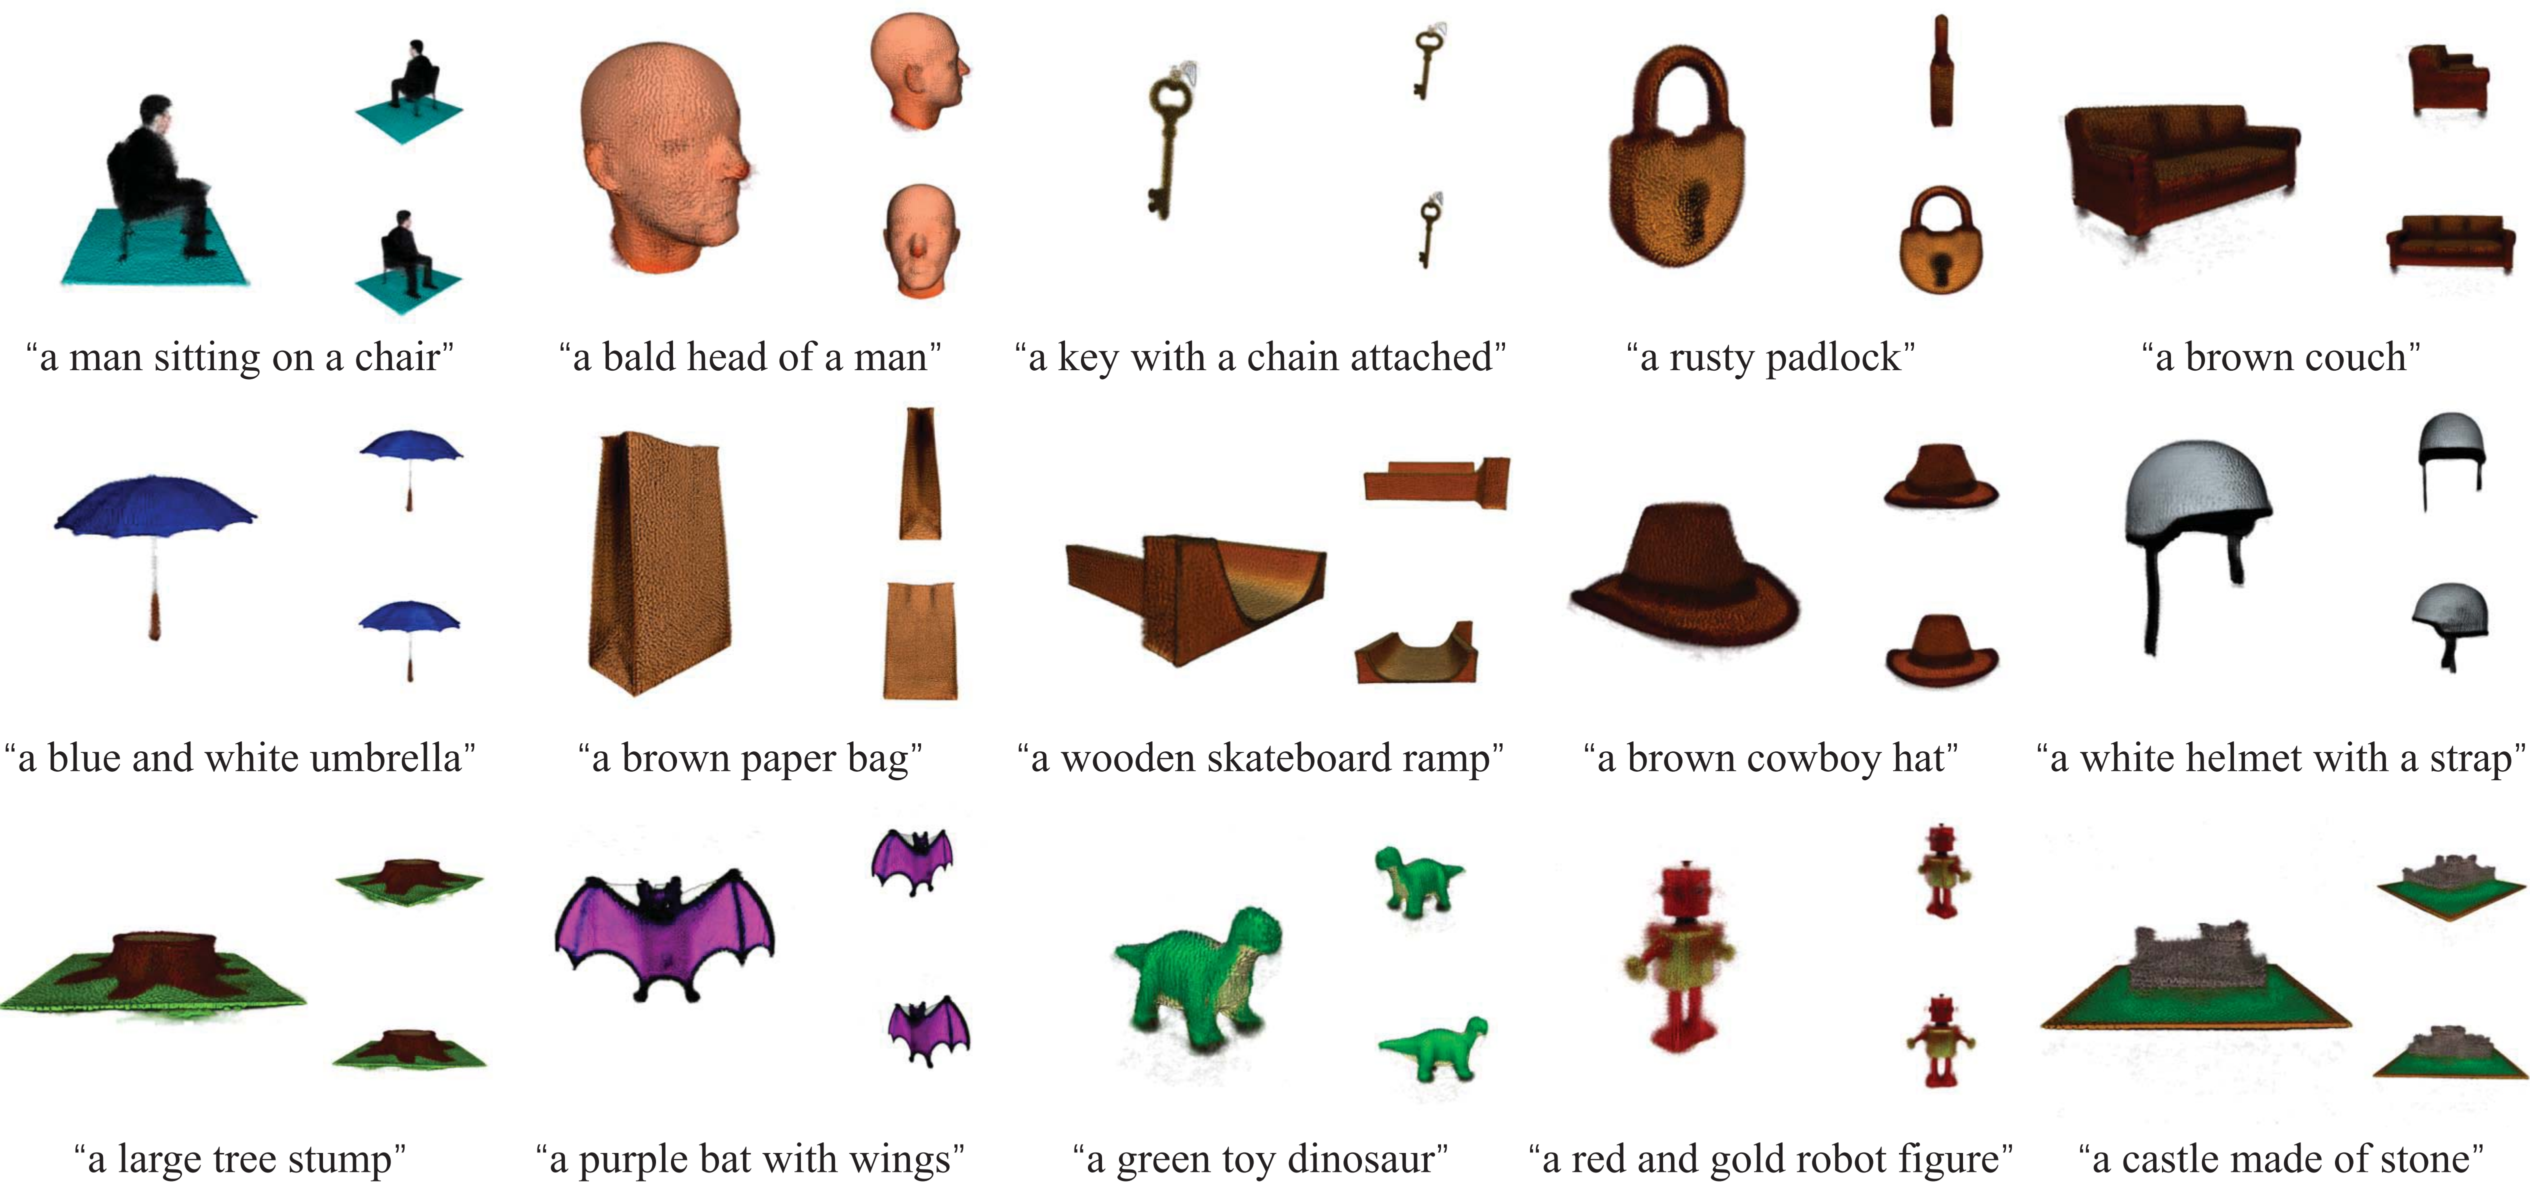
"a man sitting on a chair"
"a bald head of a man"
"a key with a chain attached"
"a rusty padlock"
"a brown couch"
"a blue and white umbrella"
"a brown paper bag"
"a wooden skateboard ramp"
"a brown cowboy hat"
"a white helmet with a strap"
"a large tree stump"
"a purple bat with wings"
"a green toy dinosaur"
"a red and gold robot figure"
"a castle made of stone"

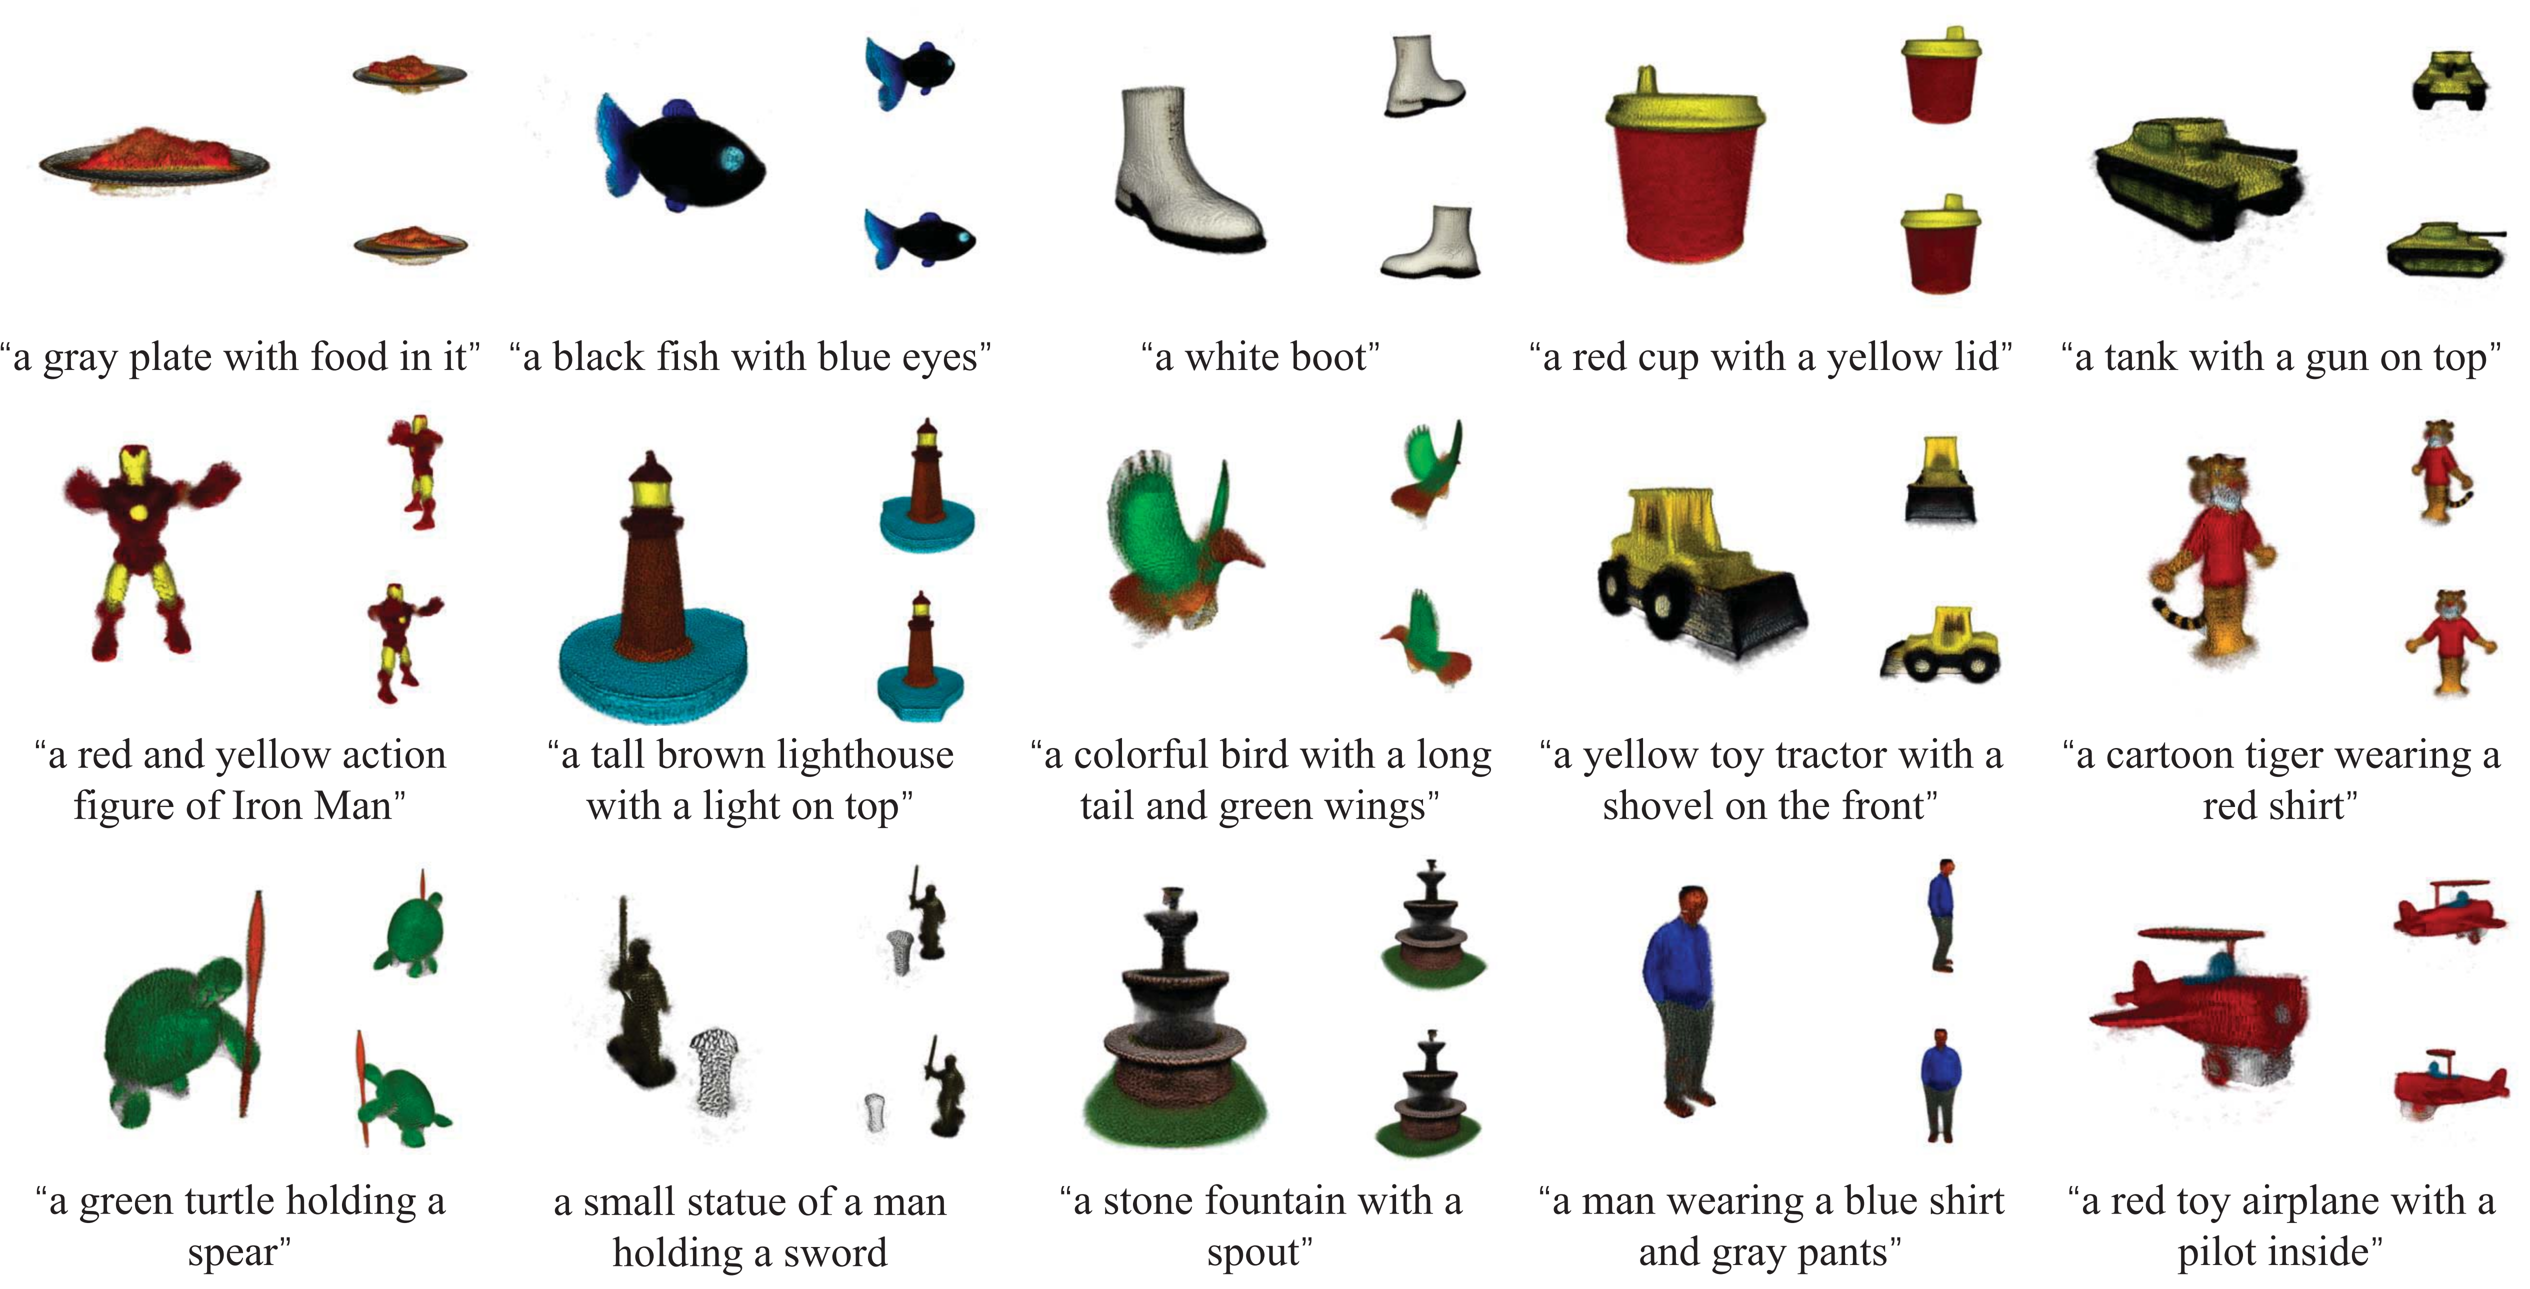
“a gray plate with food in it”
“a black fish with blue eyes”
“a white boot”
“a red cup with a yellow lid”
“a tank with a gun on top”
“a red and yellow action figure of Iron Man”
“a tall brown lighthouse with a light on top”
“a colorful bird with a long tail and green wings”
“a yellow toy tractor with a shovel on the front”
“a cartoon tiger wearing a red shirt”
“a green turtle holding a spear”
a small statue of a man holding a sword
“a stone fountain with a spout”
“a man wearing a blue shirt and gray pants”
“a red toy airplane with a pilot inside”

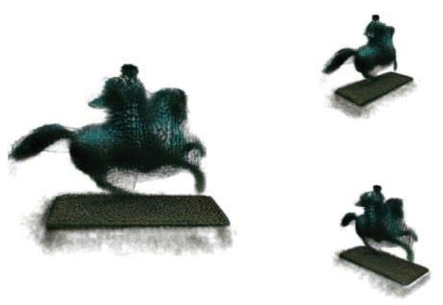

“a statue of a knight riding a horse”

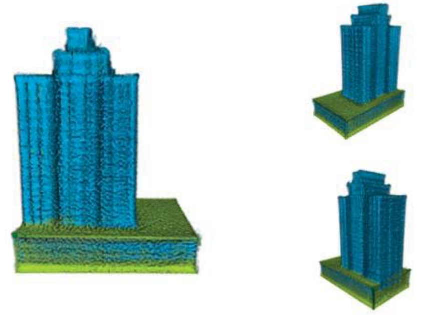

“a high-rise building with multiple floors”

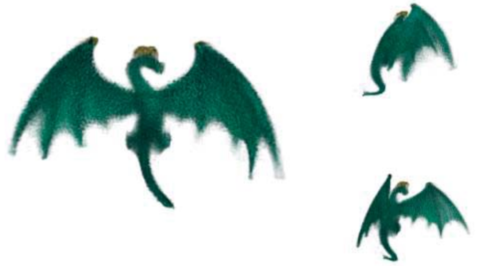

“a dragon with a crown on its head and wings”

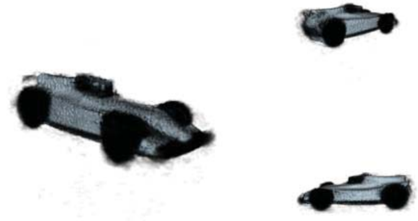

“a racing car with a silver body and black wheels”

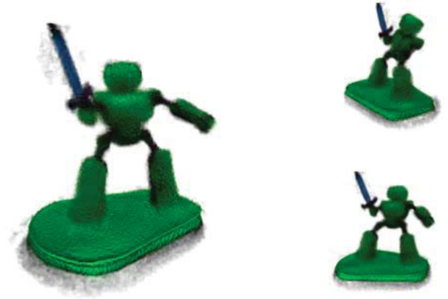

“a green robot statue with a sword in its hand”

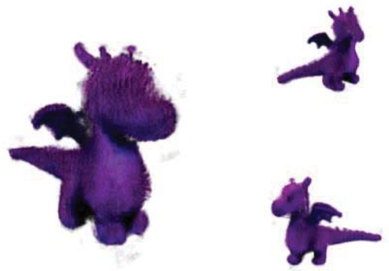

“a purple dragon toy with horns”

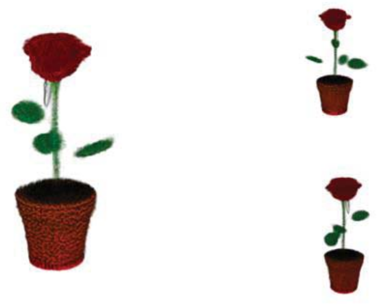

“a single red rose in a brown pot”

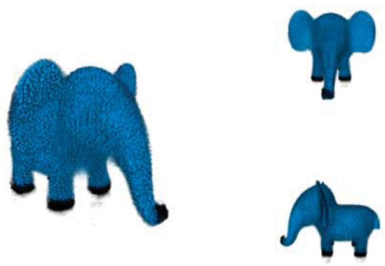

“a blue elephant with a long trunk”

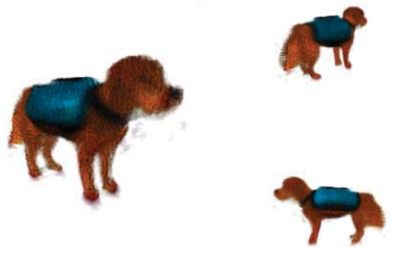

“a dog with a backpack on its back”

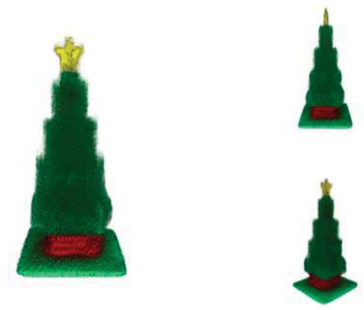

“a small Christmas tree made of Legos”

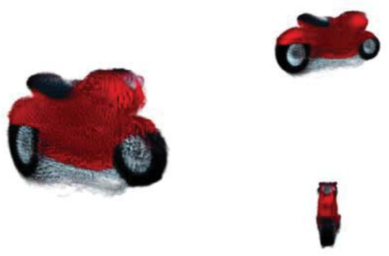

a red motorcycle with a black seat

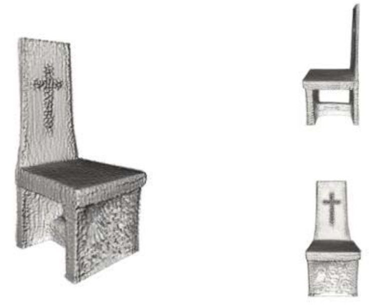

“a white chair with a cross on the back”

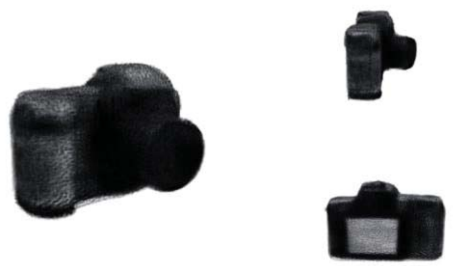

“a black and grey camera with a lens”

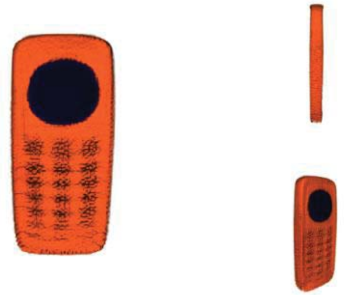

“an orange cell phone with black buttons”

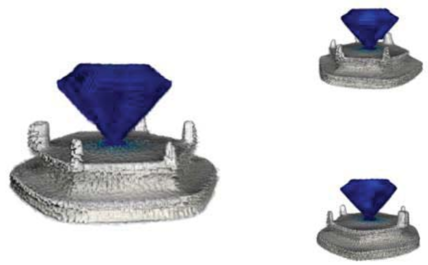

“a blue diamond on a white pedestal”

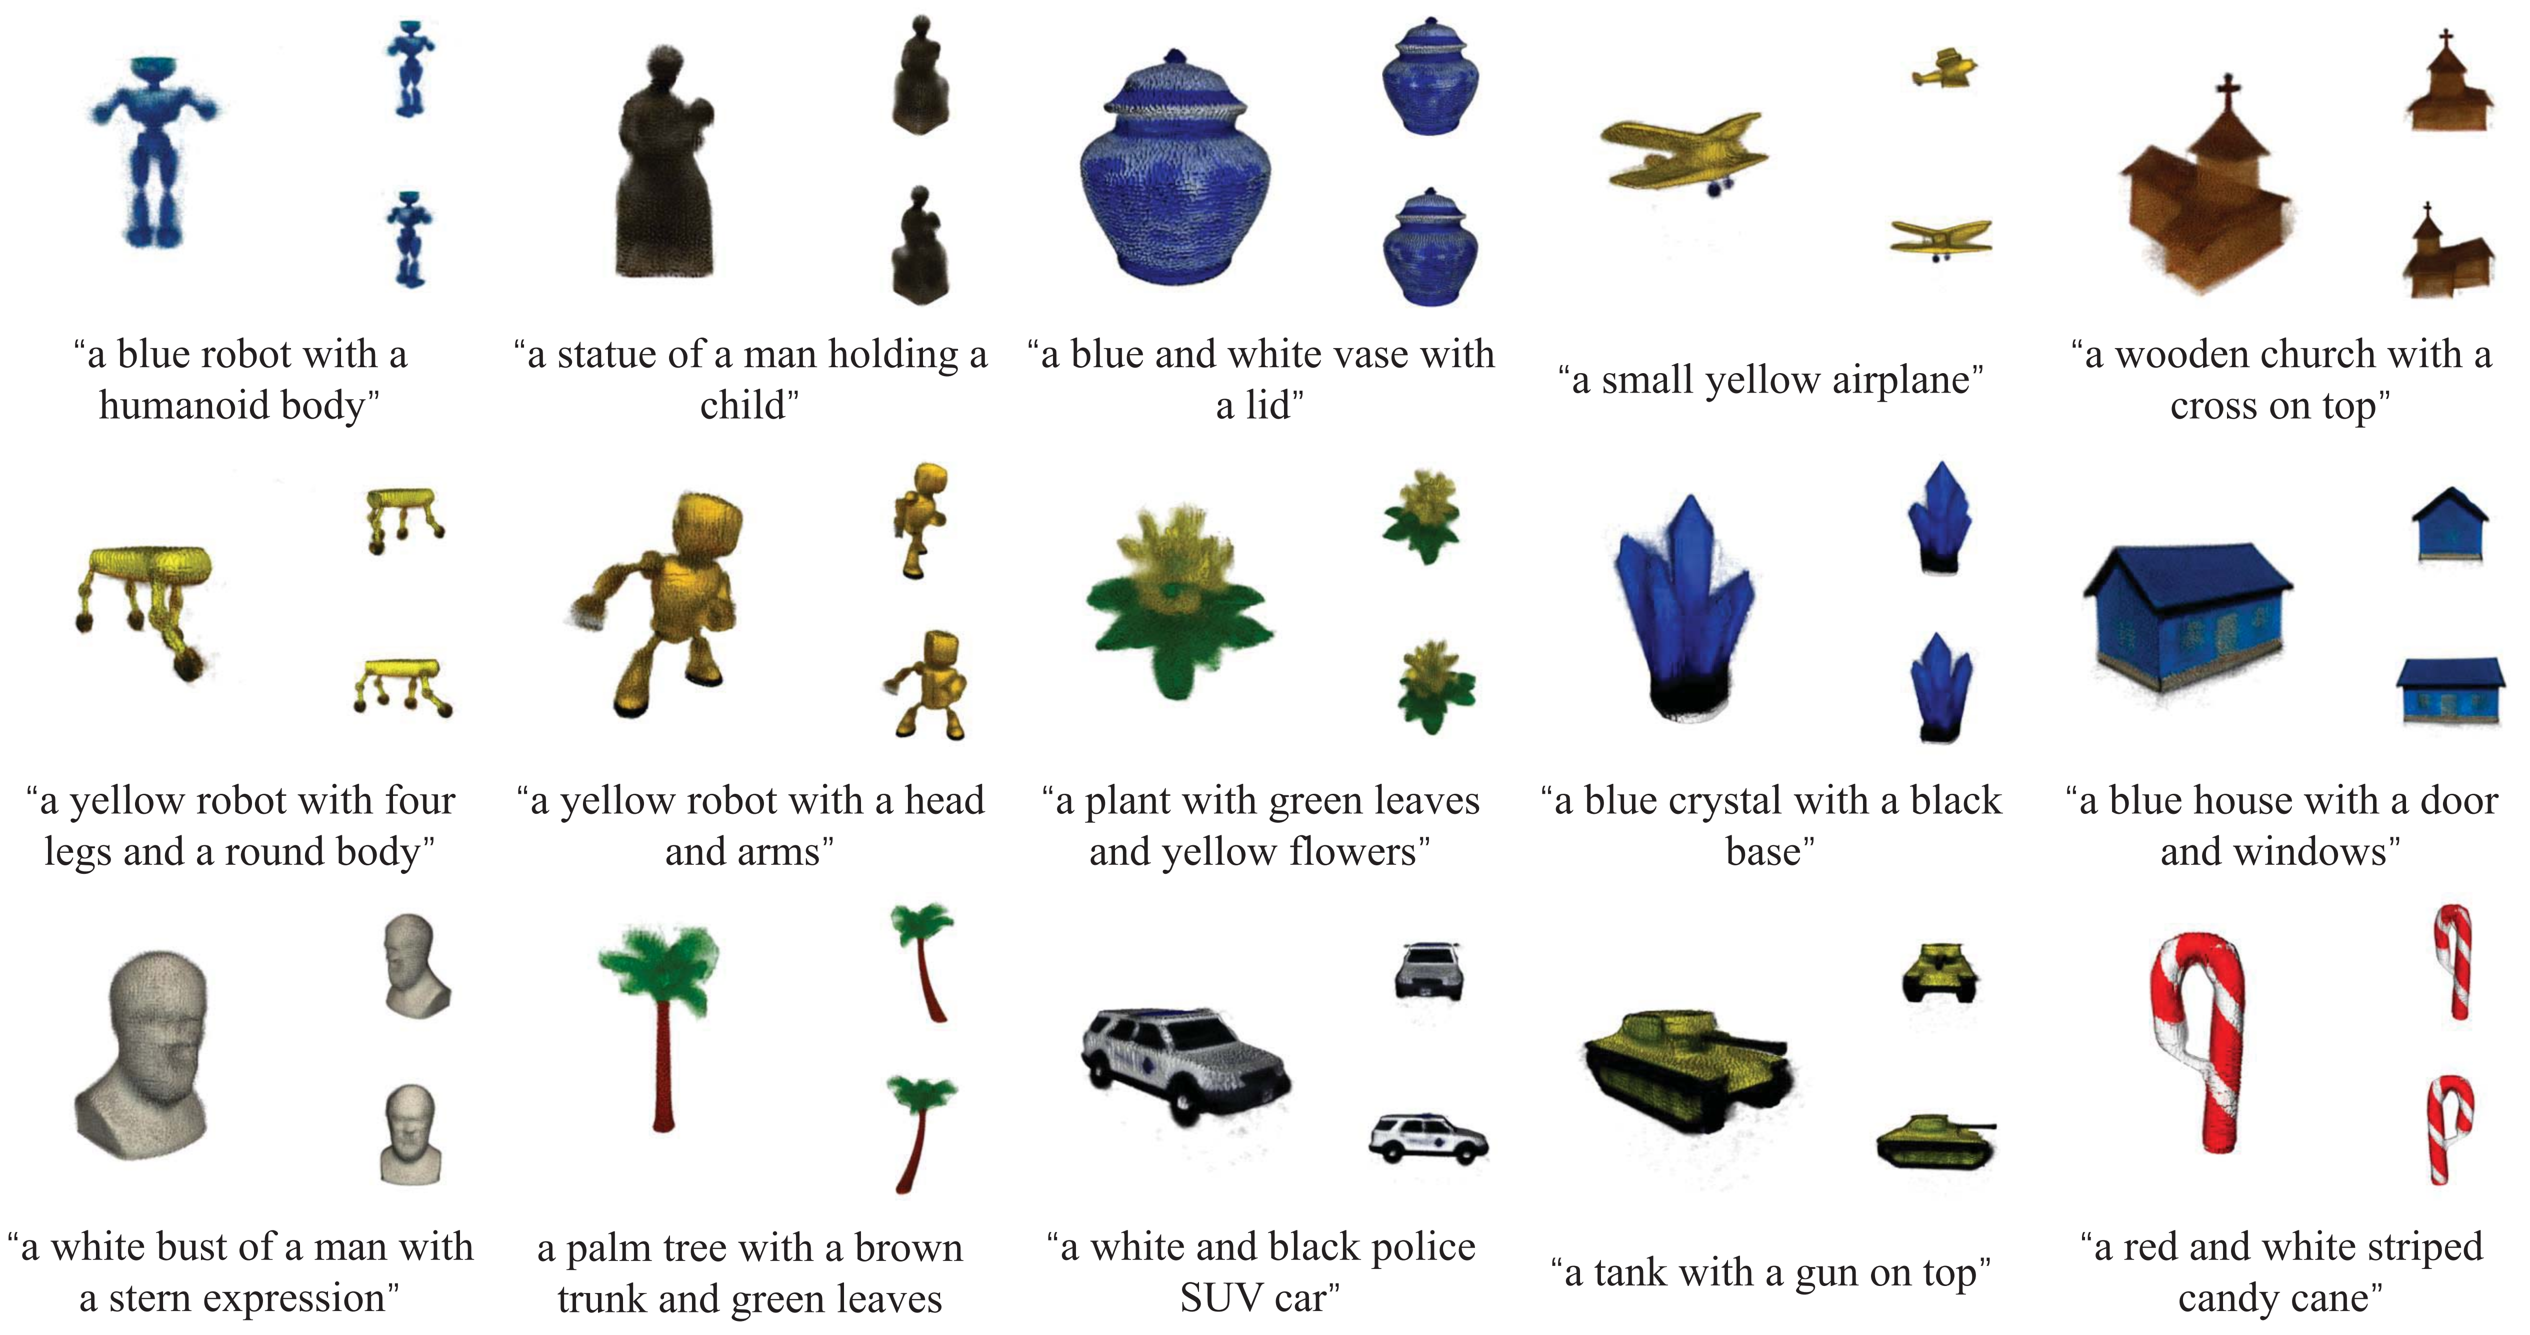

"a blue robot with a humanoid body"
"a statue of a man holding a child"
"a blue and white vase with a lid"
"a small yellow airplane"
"a wooden church with a cross on top"
"a yellow robot with four legs and a round body"
"a yellow robot with a head and arms"
"a plant with green leaves and yellow flowers"
"a blue crystal with a black base"
"a blue house with a door and windows"
"a white bust of a man with a stern expression"
a palm tree with a brown trunk and green leaves
"a white and black police SUV car"
"a tank with a gun on top"
"a red and white striped candy cane"

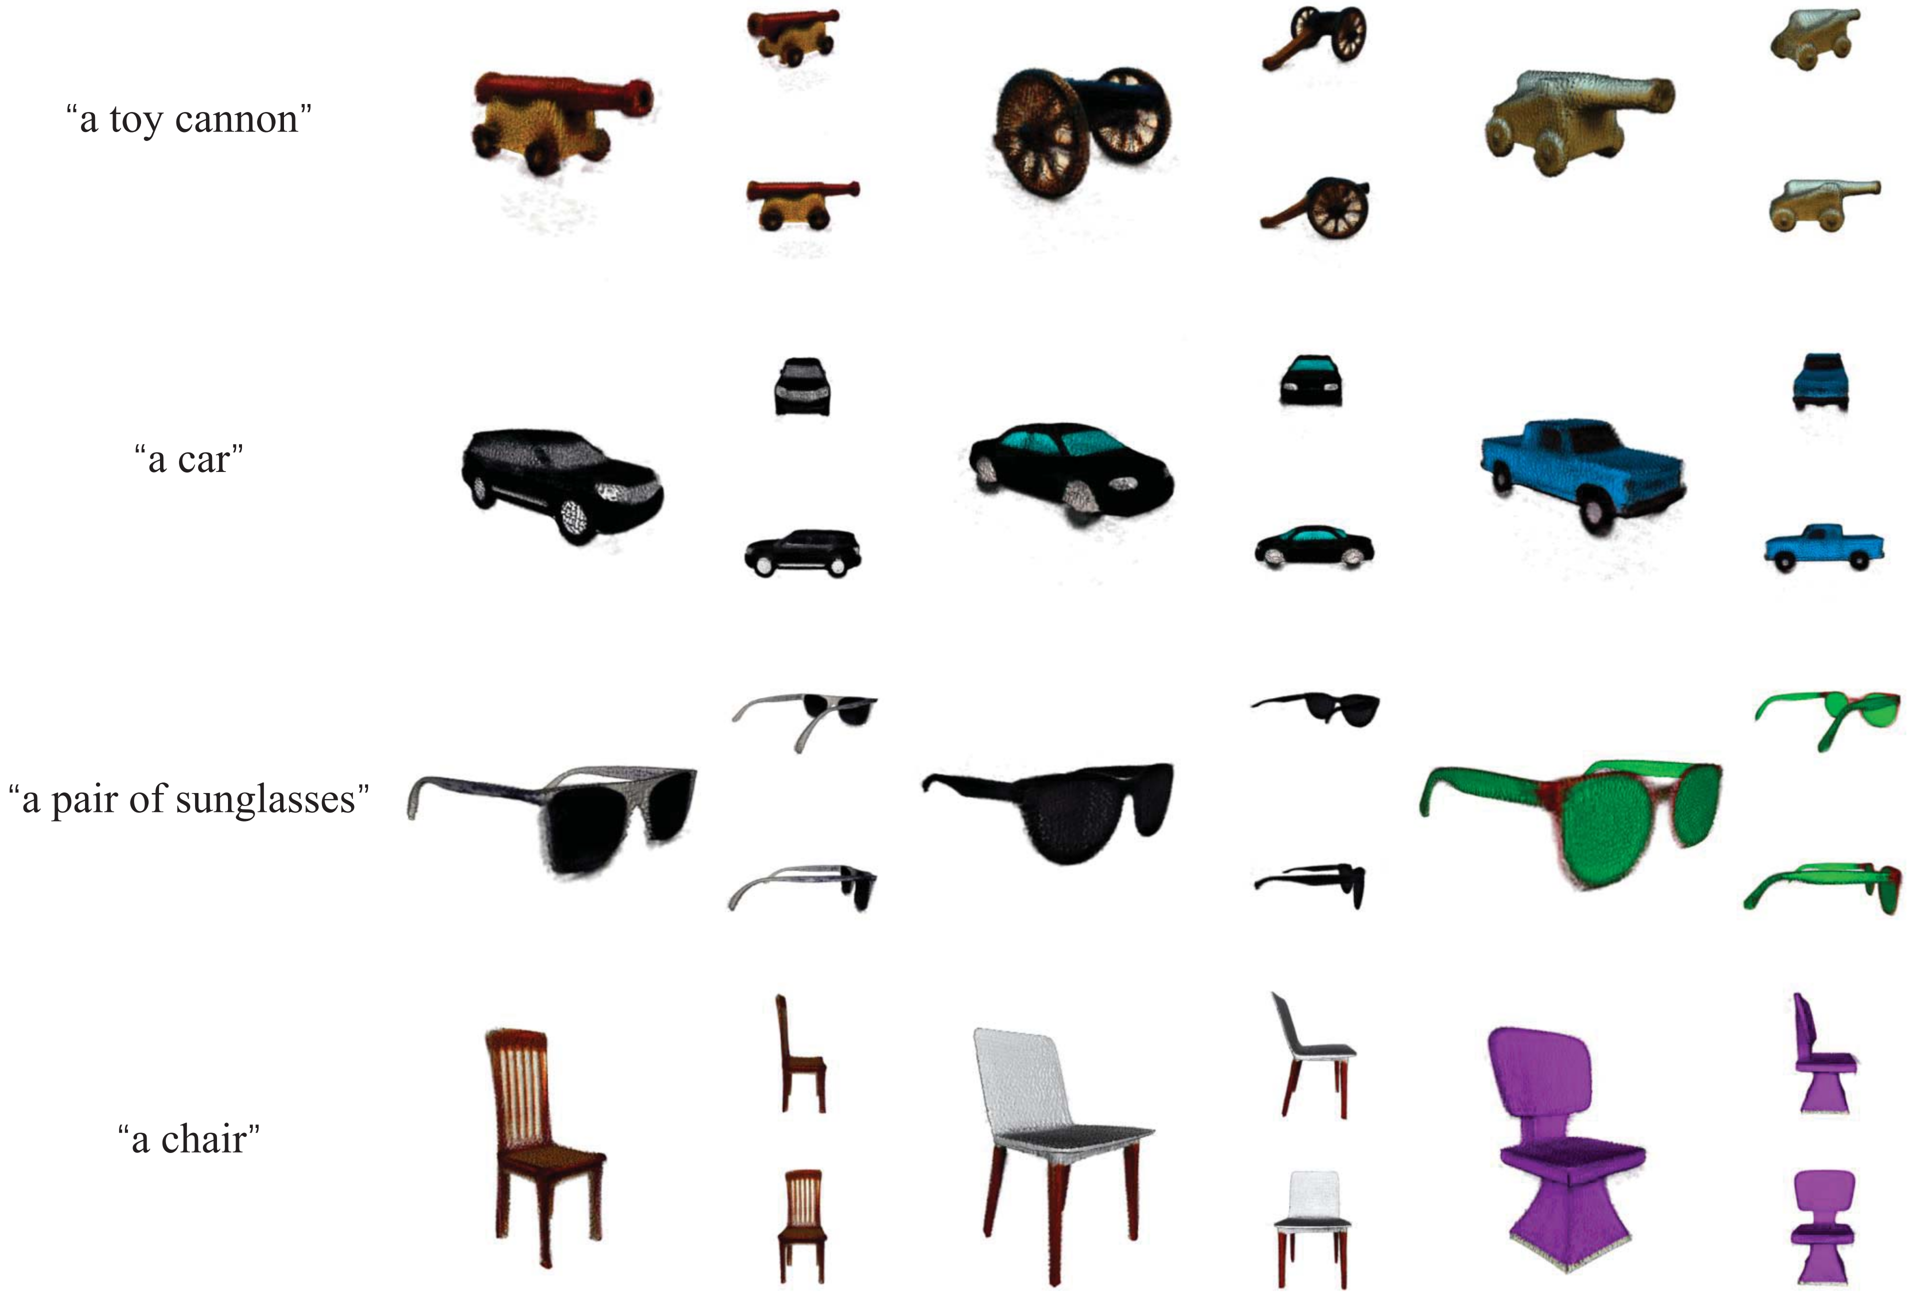
"a toy cannon"
"a car"
"a pair of sunglasses"
"a chair"

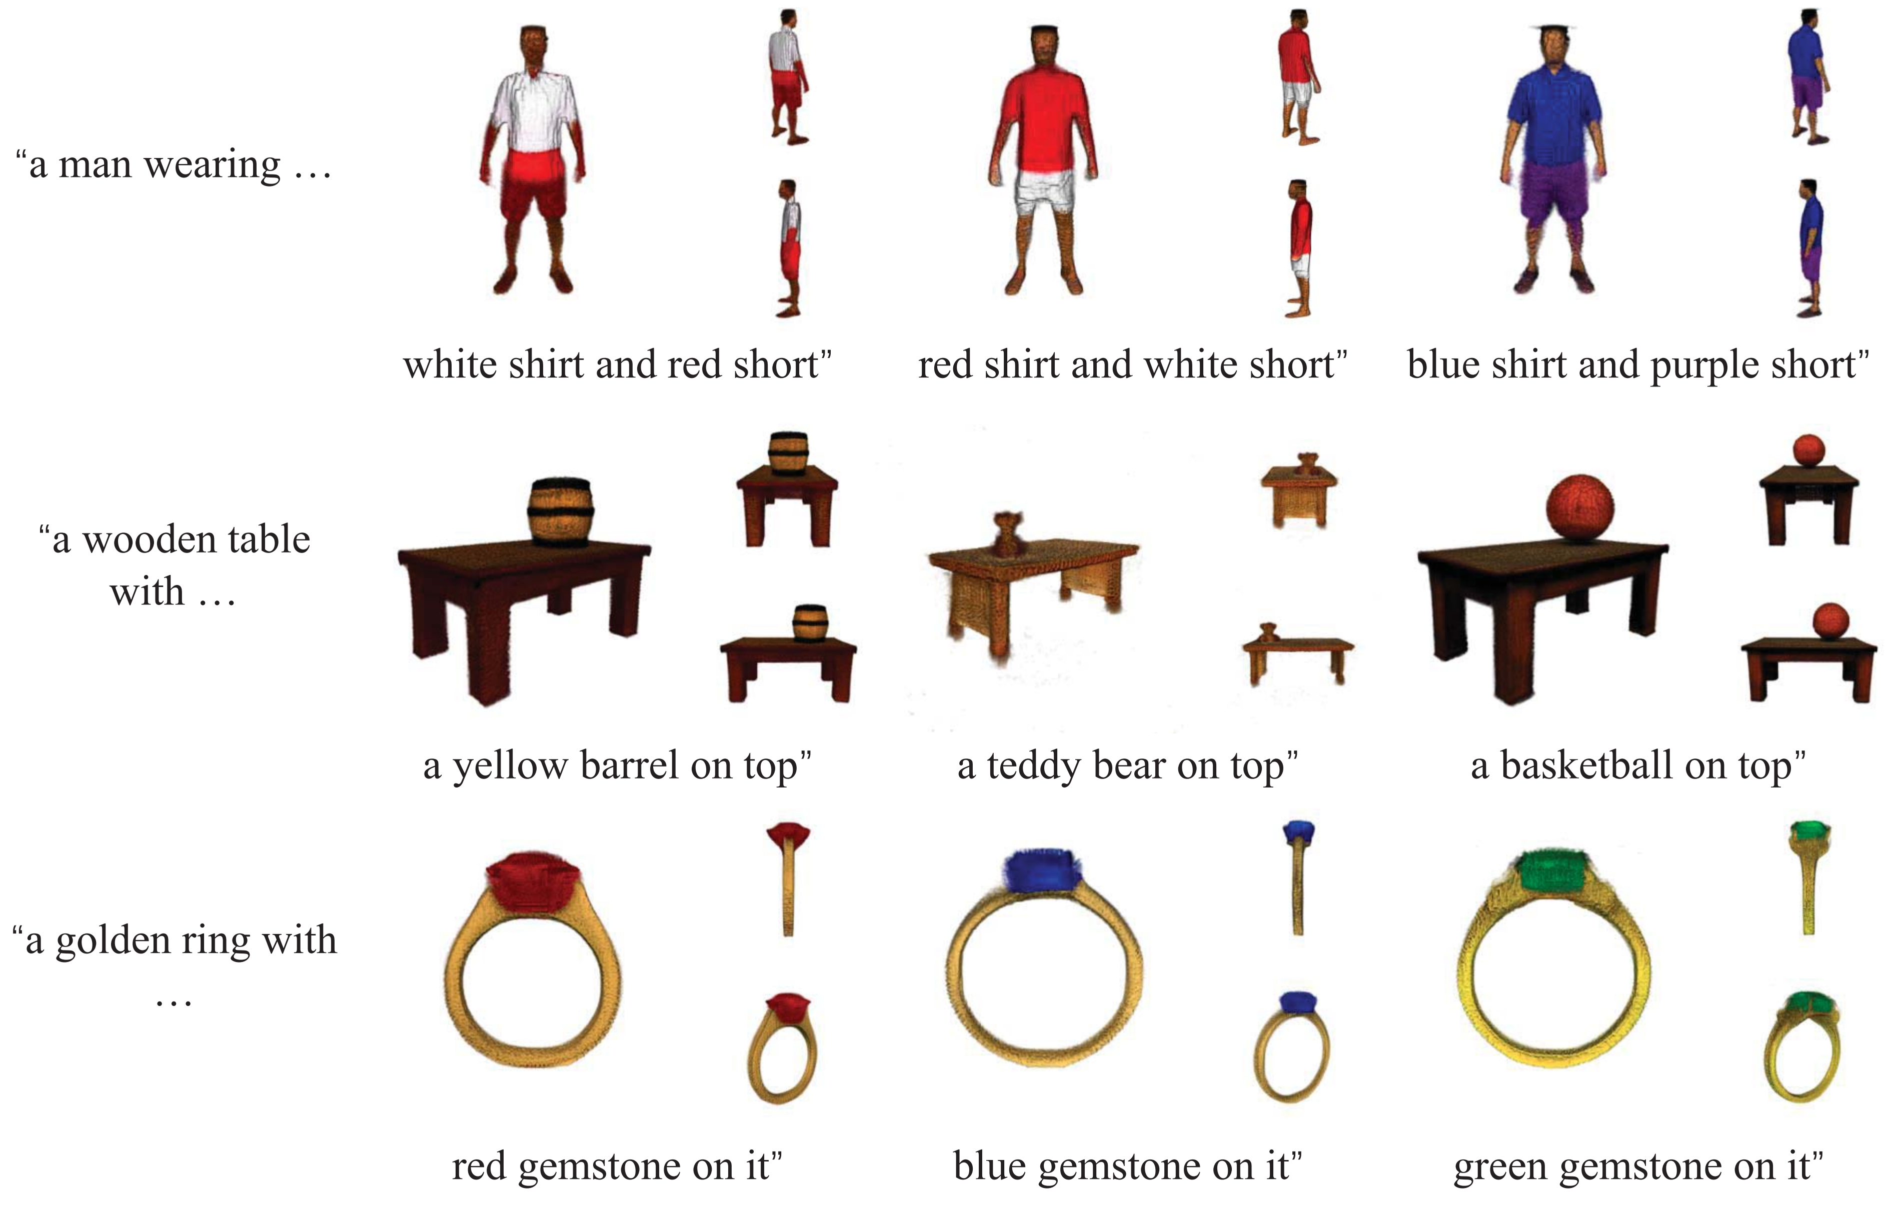

“a man wearing …
white shirt and red short”
red shirt and white short”
blue shirt and purple short”
“a wooden table with …
a yellow barrel on top”
a teddy bear on top”
a basketball on top”
“a golden ring with …
red gemstone on it”
blue gemstone on it”
green gemstone on it”

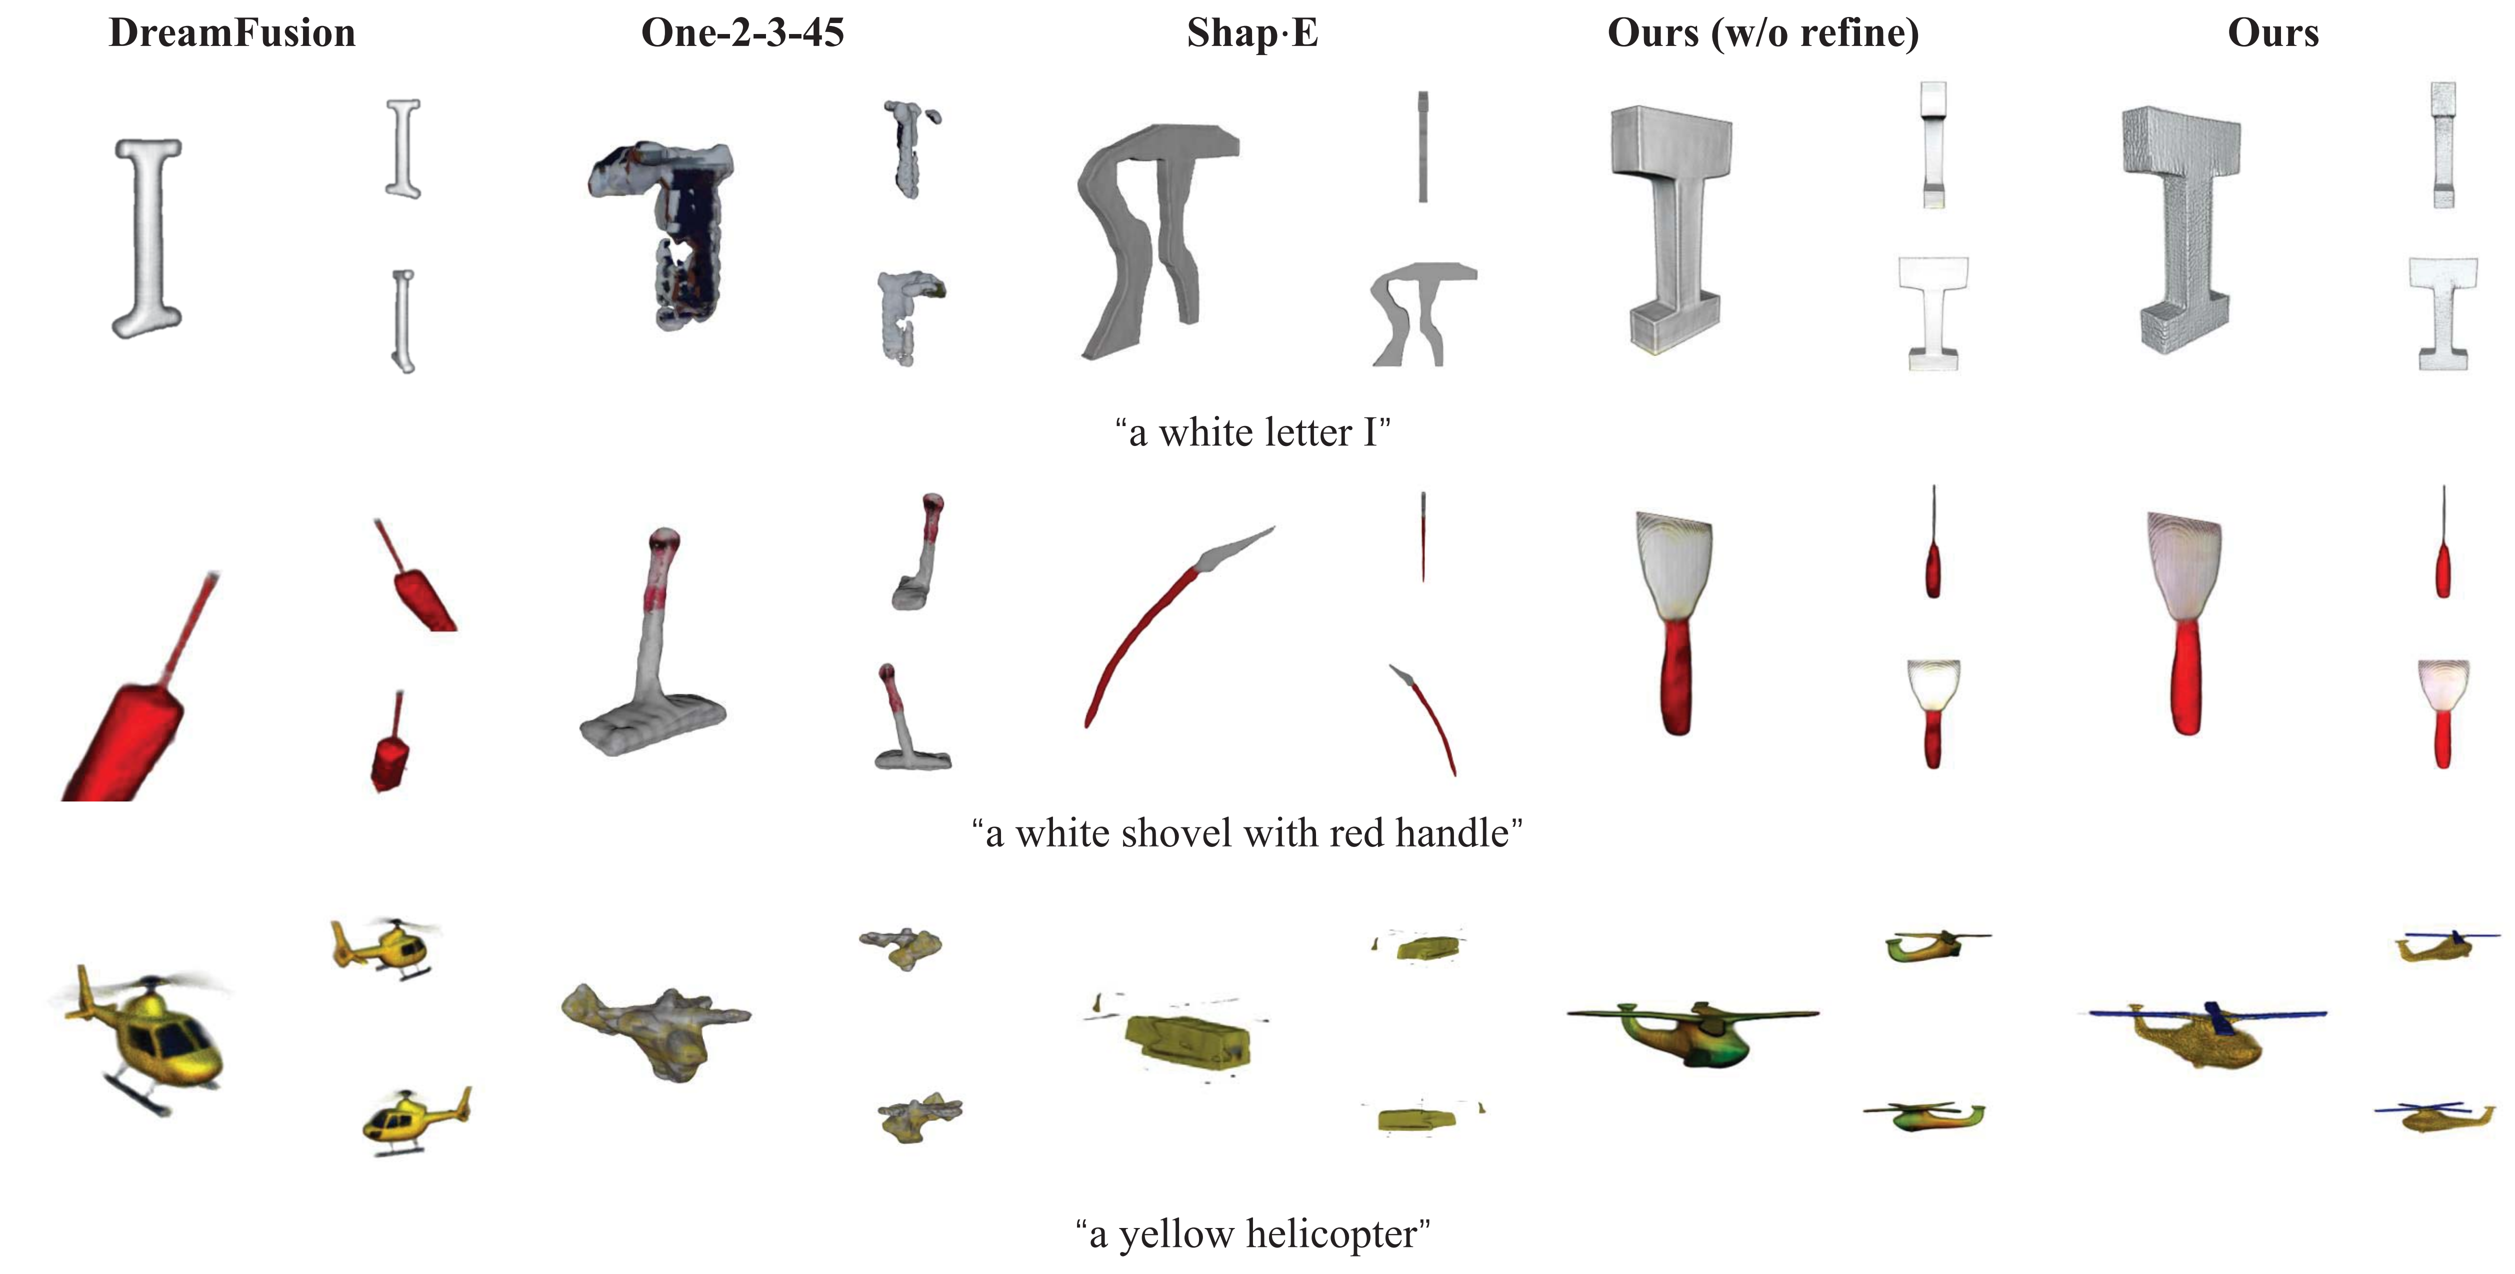
DreamFusion
One-2-3-45
Shap·E
Ours (w/o refine)
Ours
“a white letter I”
“a white shovel with red handle”
“a yellow helicopter”

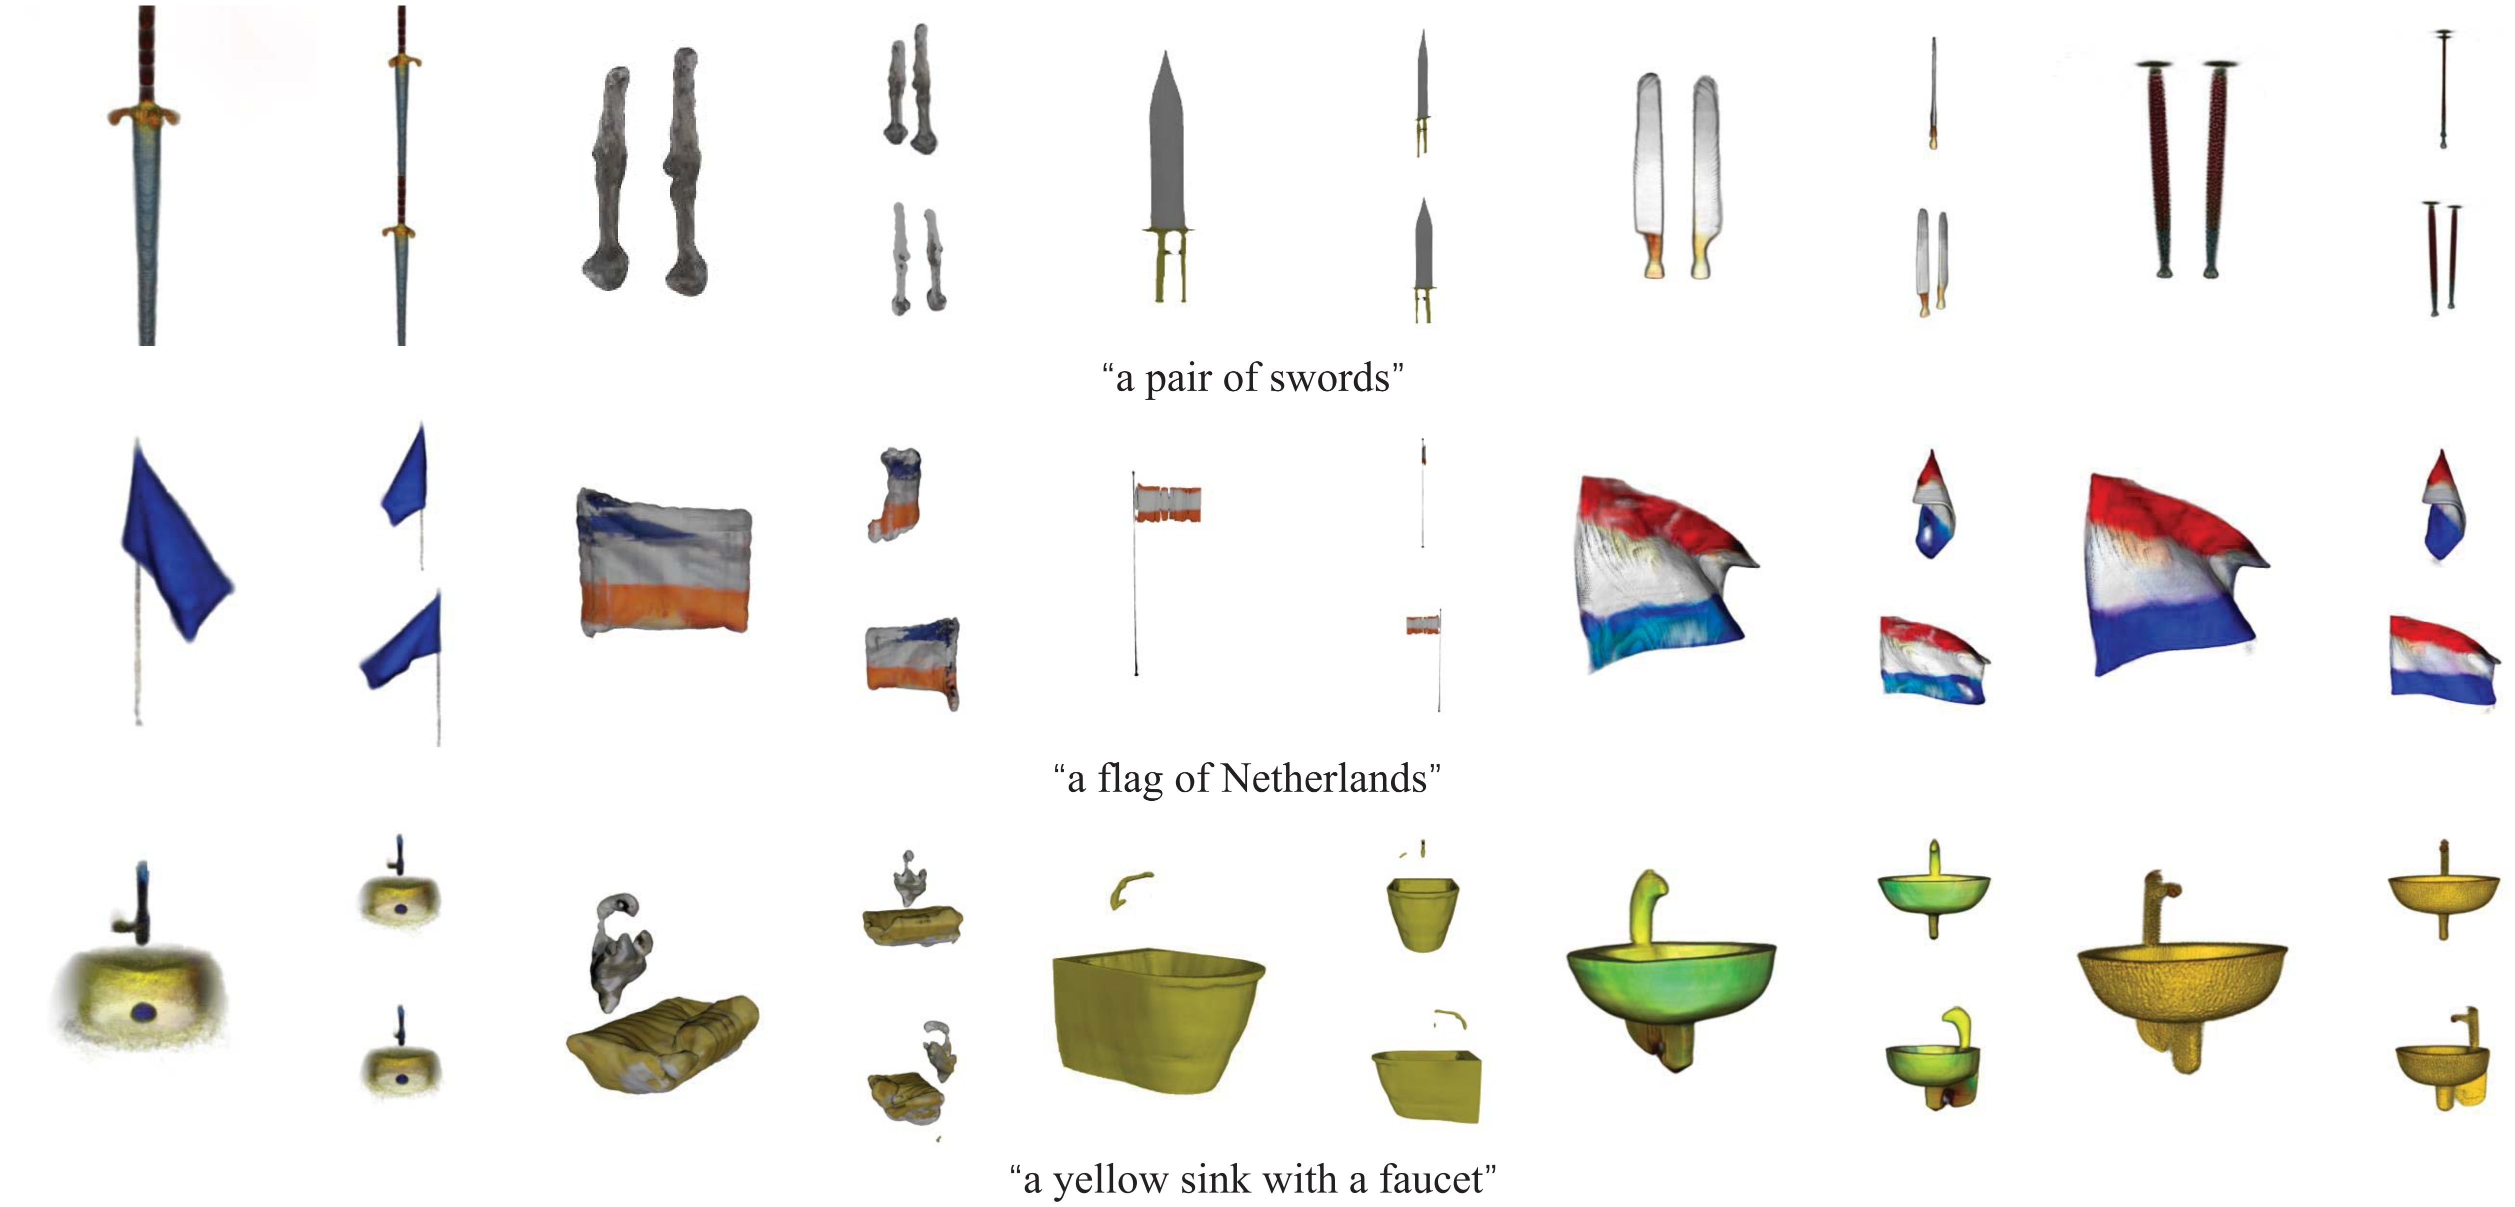
"a pair of swords"
"a flag of Netherlands"
"a yellow sink with a faucet"

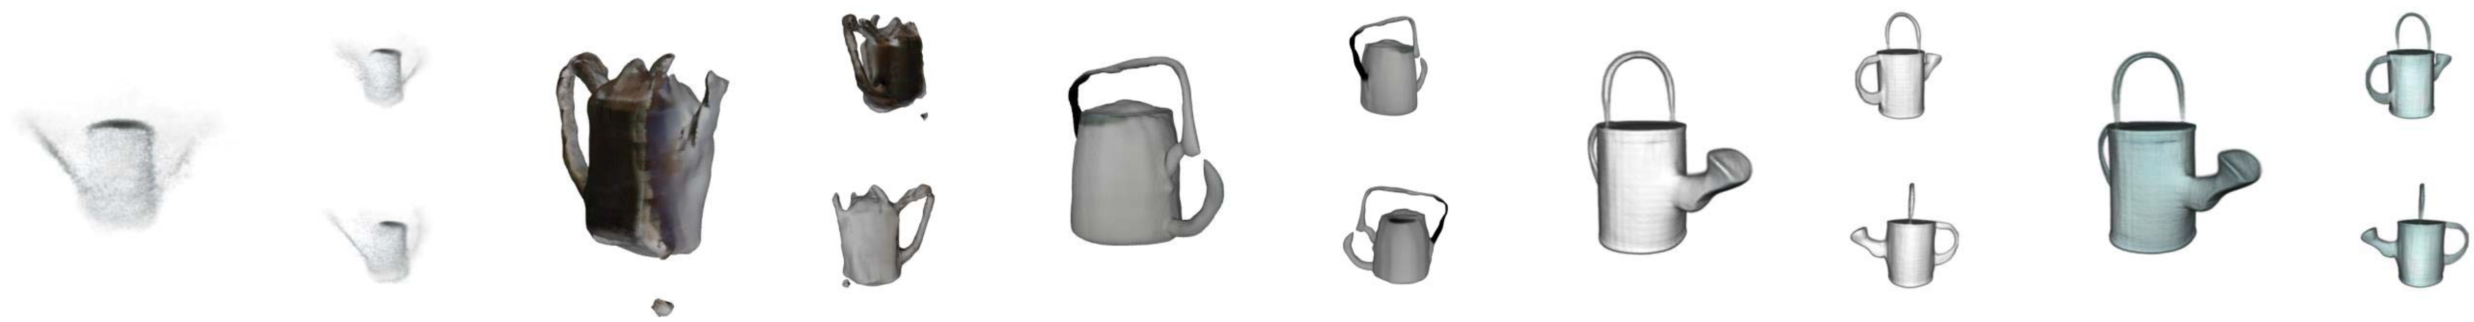

“a white watering can with a handle”
